# Supplementary material for: Reflective Decoding: Beyond Unidirectional Generation with Off-the-Shelf Language Models
Source: arXiv:2010.08566 source file (2021-12-24)
Supplement: Supplementary file 1 [file appendix_gen_paraphrase_2.tex]

\begin{table*}[t]
\small
    \centering
\begin{tabular}{l|c}
\toprule

\rowcolor[gray]{0.95} \multicolumn{2}{c}{ What are some tips for keeping ice cream from melting? }\\
\midrule
\textbf{Human} & Why does ice cream melt? how can you keep it from melting? \\
\midrule
\rowcolor[gray]{0.95} \multicolumn{2}{l}{Unsupervised}\\
\midrule
\textbf{RefDec-Top (Us)} & What's the best way to keep ice cream from melting? \\
\midrule
\textbf{RefDec-70 (Us)} & What's the best way to keep ice cream from melting? \\
\midrule
\textbf{RefDec-55 (Us)} & What's the best way to keep ice cream from melting? \\
\midrule
\midrule
\textbf{R-VQVAE} & What tips are for keeping some ice cream from melting? \\
\midrule
\textbf{CGMH-Top} & What are some arguments for keeping crude cream from? \\
\midrule
\textbf{CGMH-70} & What are some arguments for keeping crude cream from? \\
\midrule
\textbf{CGMH-55} & What are some arguments for keeping crude cream from?
 \\
\midrule
\rowcolor[gray]{0.95} \multicolumn{2}{l}{Supervised}\\
\midrule
\textbf{PG-IL} & What are some tips for ice cream from melting? \\
\midrule
\textbf{DiPS} &  How do I cure ice cream from melting? \\
\midrule
\textbf{BART} & What are some ways to keep ice cream from melting? \\
\midrule
\rowcolor[gray]{0.95} \multicolumn{2}{l}{Bilingual} \\
\midrule
\textbf{MT} & What tips are there to prevent ice from melting?  \\
\bottomrule
\end{tabular}

    \caption{Further generations for paraphrasing from all tested systems}  % 
    \label{tab:paraphrase_gen_2}

\end{table*}
