# Supplementary material for: Reflective Decoding: Beyond Unidirectional Generation with Off-the-Shelf Language Models
Source: arXiv:2010.08566 source file (2021-12-24)
Supplement: Supplementary file 2 [file appendix_0.tex]

\appendix
\section{Appendix}

\subsection{Derivation of Sampling Function}
\label{app:derivation}

%\peter{Need to change this to explain new notation (no more capital letters)}
%We start with a notational note: $P_{X|y}$ corresponds to the conditional distribution over random variable $X$, given a specific value $y$. This will generally correspond to the distribution of a forward or backward language model over text $X$ conditioning on $y$. Thus, $P_{X|y}(x)$ is the distribution over random textual variable $X$ conditioned on static context $y$. In contrast, $P(x)$ denotes the unconditional probability of text $x$ under a language model.

Here we derive the sampling function used for \method, working from a definition of similarity based on context and deriving a function that allows generation. This section is meant to supplement and expand upon \S\ref{subseq_intuitions_and_theory}. 

To begin, for correctness we use the notation $P_{c|s}$ to denote the distribution of contexts $c$ for source sentence $s$. In practice, this will be 1-sided context, for instance right-hand context $c_{rh}$. In this case, $P_{c|s}$ would be estimated by the left-to-right language model conditioned on s: $\text{\lrLM}(c|s)$. A clarifying example is included in figure \ref{fig_1} where contexts are sampled from this distribution. 

The reverse distribution $P_{s|c}$ is the opposite: going back from context \textit{towards} text. With right-hand context, this is estimated by the the reverse language model $\text{\rlLM}(s|c)$. We will begin by using the more general notation ($P_{c|s},P_{s|c}$) while considering theoretical quantities, then transition to using the language model distributions (\lrLM,\rlLM) when we are estimating these quantities in practice.


%We will proceed using right-context for reflection, but the left-context version proceeds identically but reversing the roles of left and right language models. 

%\peter{Maybe stick with the probabilities for now, and then turn them into LM distributions later?}

% \peter{Just relate $P_{c|s}$ to LM and then replace it when we're doing an estimate. And maybe go to the estimate CE first, then do the score derivation}


In \S\ref{subseq_intuitions_and_theory}, we consider the task of comparing a source sentence $s_{src}$ with another sentence $\hat{s}$. For instance, we may want to know if $\hat{s}$ is a paraphrase of $s_{src}$. Following a distributional intuition \citep{firth1957synopsis} that text with similar meaning will appear in similar contexts, we define a simple way to compare meaning
\begin{equation}
    D_{KL}(P_{c|s_{src}},P_{c|\hat{s}})
    \label{eqn:DKL_app}
\end{equation}
Where $D_{KL}$ is the Kullback–Leibler divergenc measuring the difference between the distributions $P_{c|s_{src}}$ and $P_{c|\hat{s}}$. This is a simple way to capture a notion above: we take the amount the contexts of $s_{src}$ and $\hat{s}$ differ as a proxy for their difference in meaning and connotation. 

While this equation (\ref{eqn:DKL_app}) plays the same role as equation \ref{eqn:context_divergence} in \S\ref{subseq_intuitions_and_theory}, we use the LM notation in that case, for simplicity and because we are only considering single-sided context there. Equation \ref{eqn:DKL_app} is more general.

In a paraphrase generation setting, we are most interested in selecting for contextual closeness, and therefore only need to rank between options. Therefore we will instead be working with the cross-entropy:
\begin{equation}
    \begin{split}
        H(\text{\lrLM}(c|s_{src}),&\text{\lrLM}(c|\hat{s})) \\
        &= \sum_{c} -\text{\lrLM}(c|s_{src})log(P_{c|\hat{s}}(c))
    \end{split}
\end{equation}
\noindent
which is equivalent to $D_{KL}$ up to a constant offset, and will be easier to estimate in practice. Here, the sum over $c$ indicates a sum over every possible context $c$. In practice we will use a finite sample estimate, but will use the theoretical formulation for now. 

As stated in Sec~\ref{subseq_intuitions_and_theory}, we are using this as a measure of contextual difference in meaning. For the purposes of paraphrasing, we are trying to find a sentence $\hat{s}$ that minimizes this, which is equivalent to maximizing the exponent of its negation:

\begin{equation}
    \begin{split}
        Score(\hat{s}) &= e^{\sum_{c} -P_{c|s} log(P_{c|\hat{s}}(c))} \\
        &= \prod_c P_{c|\hat{s}}(c)^{P_{c|s}(c)} \\
        &= \prod_c  \left ( \frac{P_{\hat{s}|c}(\hat{s}) P(c)}{P(\hat{s})} \right ) ^{P_{c|s}(c)}  \\
        &= a_0 \prod_c  \left ( \frac{P_{\hat{s}|c}(\hat{s}) }{P(\hat{s})} \right ) ^{P_{c|s}(c)}  \\
        &= \frac{a_0}{P(\hat{s})} \prod_c  P_{\hat{s}|c}(\hat{s})   ^{P_{c|s}(c)}  \\
    \end{split}
    \label{eqn:app_1}
\end{equation}
Note, $a_0$ is a constant factor resulting from factors of $P(c)$. We drop this for optimization. Also, $P_{\hat{s}|c}$ simply gives the distribution of text given context $c$ e.g. if $c$ is right context, this is the distribution estimated by a right-to-left language model \rlLM conditioned on $c$. %We use the random textual variable $\hat{s}$ simply to indicate that we will be measuring this distribution for generations $\hat{s}$.

The result of derivation~\ref{eqn:app_1} fits the Product of Experts model of \cite{hinton2002training}. In theory, the factor of $P(\hat{s})^{-1}$ will prioritize more context-specific paraphrases as a low probability sentence that's likely in contexts for $s$ is more related than a sentence that's generally likely (i.e. generic), but this has a few issues. For one, our estimators (language models) are not well equipped to handle very unlikely text, as they're trained on the real distribution and so spend relatively little capacity on very unlikely sequences. Second, while a less likely sentence can have higher similarity for the reasons stated above, this may not be the goal of our system.

In a real setting, we are interested in related sentences that are also \textit{fluent} and \textit{reasonable}. For this reason, we drop the $P(\hat{s})^{-1}$ term when calculating our approximate score, the equivalent of multiplying in $P(\hat{s})$ which is simply biasing the model towards likely sequences. 
%From the logical \peter{I should look for somewhere to cite this from...} perspective in which a product-of-experts is related to the ``and'' operation, this is essentially saying, $s_b$ should be semantically similar AND likely.

This gives an augmented score: 

\begin{equation}
    \begin{split}
        Score(\hat{s})
        &= c_0 \prod_c  P_{\hat{s}|c}(\hat{s})^{P_{c|s}(c)}  \\
    \end{split}
\end{equation}

Optimizing this is equivalent to taking a product of experts of the following form:

\begin{equation}
    \begin{split}
        Score(\hat{s}) 
        &= \prod_c  P_{\hat{s}|c}(\hat{s})^{w_{c|s}}  \\
    \end{split}
    %\label{eqn:app_PoE_score}
\end{equation}

There is then the question of how we should set the weights $w_{c|s}$ in the limited sample setting. In the full setting, these weights are a set of probabilities $P_{c|s_{src}}(c)$ summing to 1 over all contexts c. This indicates the logarithm of the score corresponds to a convex combination of the logits of the distributions $P_{\hat{s}|c}(\hat{s})$. To keep in line with this notion, we will also enforce that weights constitute a proper distribution. 

In the limiting case with unlimited samples, these weights should be set to the probability of context given $s$, $P_{c|s}(c)$. A simple method to take this to the finite-sample case would be simply renormalizing these probabilities given over the sampled contexts. However, it is not clear that these are the most efficient weights for a good estimate of the scoring function. Further, while pretrained LMs are strong estimators, exponentiating by their estimates will magnify any errors they make. Instead, we learn these weights using a heuristic, discussed later.

As we transition to the finite-sample-setting and consider estimating this in practice, we replace the theoretical distributions with estimates using language models. In doing so, we go from a more general notion of context to 1-sided. Here we will consider right-context (meaning $P_{\hat{s}|c}$ is estimated by \rlLM) but the left-context case proceeds symmetrically. Substituting in the language model distribution:

\begin{equation}
    \begin{split}
        Score(\hat{s}) 
        &= \prod_c  \text{\rlLM}(\hat{s}|c)^{w_{c|s}}  \\
    \end{split}
    \label{eqn:app_PoE_score}
\end{equation}

Where now the product over $c$ indicates product over the finite sampled contexts. We will discuss how the weights are learned, but first we convert this to a sampling function. We can now decompose the scoring function into tokens of generation $\hat{s} = \hat{s}_0 ... \hat{s}_n$:

\begin{equation}
    Score(\hat{s}_{0:n}) = \prod_{j} \prod_c  \text{\rlLM}(\hat{s}_j|\hat{s}_{j+1:n})^{w_{c|\hat{s}}}
\end{equation}

This is simply restating equation~\ref{eqn:app_PoE_score} but factorizing LM probability by tokens. 

Renormalizing and decomposing by token position, this gives a natural distribution to sample from:
\begin{equation}
    \begin{split}
            P_{sample}&(\hat{s}_j|\hat{s}_{j+1:n}) = \\ & \frac{ \prod_c  \text{\rlLM}(\hat{s}_j|hat{s}_{j+1:n})^{w_{c|s}}}{ \sum_{t \in V}  \prod_c  \text{\rlLM}(t|hat{s}_{j+1:n})^{w_{c|s}} }
    \end{split}
    \label{eqn:rd_appendix}
\end{equation}
Simply, we are normalizing at each point over tokens in the vocabulary $V$, making this a proper token-wise distribution to sample from. Note that we are sampling right-to-left, so from index $n$ down, to match convention. This is the sampling function referred to as \rlRD in the body of the paper, and state in equation \ref{eqn:rd_theory}. We use this to sample candidate generations that encourage adherence to the semantic scoring function. Note, in practice we refer to contexts by index $i$ ($c_i$) and the associated weight as $w_i$.

Finally, we learn the weights, following the convex combination constraint (weights are nonnegative, summing to 1), to match one fundamental aspect of the scoring function. That is, $s_{src}$ should receive the highest score (or similarly, should have the lowest contextual difference with itself). So essentially, we learn weights that maximize the score/probability of $s_{src}$, using a gradient-based learning algorithm to achieve this. This assures that the entire algorithm can proceed using only the two language models and input, as the signal for learning comes only from the self-generated context and input. 

\section{Implementation Details}
\label{app:implementation}

\subsection{Left-to-Right \decoder}
\label{app:lr}

As mentioned in \S\ref{subsec:reflective_decoder}, a left-to-right \decoder \lrRD is learned in a similar manner to \rlRD, simply by switching the roles of \lrLM and \rlLM in algorithm \ref{alg}. For completeness we elaborate on this here. 

First, the roles of the language models are flipped in the sampling function:


\begin{equation}
    \text{\lrRD(s)}= \frac{ \prod_i \text{\lrLM}(s|c_i)^{w_i}}{ \prod_{j=0}^{|s|} \sum_{t \in V}  \prod_{i}  \text{\lrLM}(t|s_{0:j-1} + c_i)^{w_i} }
    \label{eqn:rd_lr}
\end{equation}

where contexts $c_i$ are now generated by the right-to-left language model \rlLM (i.e. left-contexts). We then present algorithm \ref{alg_lr}, which defines how to learn \lrRD.

\input{figs/algorithm_lr}


\subsection{Post-processing Generations} Without learning stop-tokens, \method samples fixed number ($len_{\hat{s}}$) of tokens. Candidates are extracted from raw generations using sentence tokenization to trim extra text to the sentence boundaries. 

\subsection{Entropy Calibration}
\label{app:entropy_calibtration}

Entropy calibration is used when sampling candidate generations (\S\ref{subsec:implementation}). We define this here.

When sampling output generations, generation parameters (truncatoin parameter $p_{\hat{s}}$ from nucleus sampling, in paraphrasing) control how ``greedy'' or stochastic the sampling process is. However, the exact effect of a specific value of $p_{\hat{s}}$ depends on target length, number of generated contexts, complexity of meaning, desired level of agreement with source etc. Setting $p_{\hat{s}}$ too low may sample only the most likely option, but too high can result in off-topic candidates. Simply, the ``correct'' value of $p_{\hat{s}}$ is highly sample-dependent.

Instead, we define a technique, \textbf{entropy calibration}, designed to control how much ``randomness'' is used in sampling in a more robust way. Rather than directly setting a $p_{\hat{s}}$ for all examples, entropy calibration allows the user to specify the amount of randomness or approximate entropy $\hat{h}$ they would like to sample with for each example. In the greedy case for instance, the desired entropy $\hat{h}$ is set to 0, or equivalently we are picking from a set of 1 possible option. Likewise, the user might set $\hat{h}$ to 4, which would result in a higher $p_{\hat{s}}$ (how much higher will be example-dependant). 

In practical terms, we search for $p_{\hat{s}}$ in each case that is expected to give the correct level of ``randomness'' over the entire generation, although $p_{\hat{s}}$ is a token-level parameter. To estimate how random a given value of $p_{\hat{s}}$ will make a generated sentence, we take the sampling entropy over the source text $s_0...s_n$ under the nucleus-sampling truncated distribution P$_p$:
$$\hat{h} = \sum_i \sum_{w \in V_p} -P_p(w|s_0 ... s_{i-1}) \text{log} P_p(w|s_0 ... s_{i-1}) $$

Where $V_p$ is the truncated vocabulary with parameter $p$. Roughly, this captures a branching-factor over the sequence. We select $p_{\hat{s}}$ that gives a desired entropy. We set this to values of 4 or 6 which we found effective. Parameters are available in App.~\ref{app:model_params}.

\subsection{Parameters}
\label{app:model_params}
In this section, we outline model settings for our 2 experimental settings, paraphrasing and $\alpha$NLG. See Table~\ref{tab:params}. 

Broadly, $\alpha$NLG achieves higher variety in output with a higher sampling entropy ($h_{sample}$), more diverse generated contexts (higher $p_c$), and fewer generated contexts ($n_c$).

To find these parameters, we experimented with different reasonable values on the dev set of each model, and evaluated manually whether generated text appeared reasonable, specifically reading examples and picking model settings that produced good paraphrases as judged by the authors. For $len_{\hat{s}}$ and $len_{h}$ we simply set this high enough to ensure desirable outputs would be a subsequence. 

We trained our transformer language models on TPU pods (using code in TensorFlow) of size 512 until convergence. These are general purpose and will only need to be trained once; they will be made publicly available. During our generation experiments, we transferred the model to Pytorch, and ran locally on a machine with 2 NVIDIA Titan Xp GPUs. 

\input{figs/model_params}

\section{Evaluation}


\subsection{Automatic Metrics}
\label{app:auto_metrics}
Links to the code we used for automatic evaluation are given here:

\begin{itemize}
    \item \href{https://pypi.org/project/pyrouge/}{ROUGE}
    \item \href{https://www.nltk.org/_modules/nltk/translate/bleu_score.html}{BLEU}
    \item \href{https://www.cs.cmu.edu/~alavie/METEOR/README.html}{METEOR}
    \item \href{https://github.com/snover/terp}{\TERP}
    \item \href{https://github.com/cocoxu/simplification/blob/master/SARI.py}{SARI}
    \item \href{https://github.com/Tiiiger/bert_score}{BERTScore}
    \item \href{https://github.com/google-research/bleurt}{BLEURT}
\end{itemize}

\noindent
We include a limited number of metrics in the main paper for space and clarity, but include further metrics tested in table \ref{tab:quoratest_aux}: ROUGE-1, ROUGE-2 \citep{lin-2004-rouge}, BLEURT \cite{Sellam2020BLEURTLR}, BERTScore \citep{Zhang2020BERTScoreET}. For BLEURT, we used the "BASE" pretrained model suggested by the authors. For BERTScore, we use the default settings of the official codebase. We also include the iBLEU metric of \citet{sun-zhou-2012-ibleu} with parameter $\alpha=0.9$.

\input{figs/quora_results_aux_metrics}

\subsection{Human Evaluation}
\label{app:human_metrics}
For human evaluation on the Quora paraphrasing corpus, we evaluate on 200 input sentences, having 3 raters evaluate each model's output. We ask about fluency, consistency with the source, and difference in wording from the source (template in figure \ref{fig:paraphrasing_template}). In each case, we use a multi-point likert scale, but are mainly interested in whether generations meet a threshold for each criterion: fluent enough to understand, with at most minor differences in meaning and at least minor differences in wording. In table \ref{tab:quora_human} we give the rate for each model that humans found generations meet these thresholds. The ``Overall'' column is the rate that humans find generations meet all 3 measured criteria. We take Fleiss' $\kappa$ on these binary combined categories (following \citet{combine_irr}) finding agreement of 0.4 (fluency), 0.54 (consistency), 0.77 (wording), and 0.48 (overall) indicating moderate to substantial agreement \citep{landis1977measurement}.

On the Twitter URL corpus, we evaluate on 100 examples, on a reduced set of models (unsupervised and MT). Besides this, the setup is the same as Quora. These results are in table \ref{tab:twitter_human}. We find agreement of 0.39 (fluency), 0.42 (consistency), 0.54 (novelty), and 0.36 (overall) indicating fair to moderate agreement.

As stated in \S\ref{sec_experiments}, for $\alpha$NLG over 1000 examples we have 3 raters on Amazon Mechanical Turk evaluate each model. We ask about agreement between h and $o_1$, $o_2$, both, and overall quality on 4-value likert scales. We found Fleiss' kappa of 0.31, 0.29, 0.28, and 0.30 respectively, indicating fair agreement which is reasonable given the large number of options.

The template used for $\alpha$NLG is in figure \ref{fig:anlg_template}, and for paraphrasing in figure \ref{fig:paraphrasing_template}.



\input{figs/quora_human}


\subsection{Twitter Dataset}
\label{subsec_twitter}
We include here the full results for our secondary paraphrasing evaluation on the Twitter URL corpus \cite{lan2017continuously}, a set of paraphrase pairs created by linking tweets with matching shared URLs validated by human judges. This marks a significant domain shift from our primary paraphrasing task (question paraphrasing). We test the most comparable baselines to \method, mainly unsupervised models CGMH and R-VQVAE as well as the backtranslation MT model. These are all described in detail in \S\ref{subseq_quora_gen}. R-VQVAE, the MT model, and \method do not use corpus-specific training data. CGMH trains on un-paired sentences from the Twitter training set, as outlined in the original work \cite{miao2019cgmh}. For all models, we use the same parameters as on the Quora dataset. 

While we include SARI, Human, and $Novelty$ in the main paper, here we include results on a number of automatic metrics (table \ref{tab:twitter_results}). Results are similar to Quora: a novel setting of Reflective Decoding (in this case RD$_{45}$) achieves the highest score on SARI, which seemed most aligned with Human on Quora and is the only metric included here that accounts for both novelty and quality. The metrics that do not account for novelty are unsurpisingly dominated by generations with lower novelty: $RD_{Top}$ gets the highest unsupervised BLEU (MT is highest overall), while R-VQVAE gets the highest unsupervised METEOR and CGMH$_{Top}$ the best unsupervised TER$_P$. 

We also include full human results in table \ref{tab:twitter_human}.

\input{figs/twitter_results}

\input{figs/twitter_human}

\subsection{Reflective Scoring Evaluation}
\label{subsec_wmt18}
While the effectiveness of sampled contexts as a representation for paraphrasing is supported by our main experiments (\S\ref{sec_experiments}), we would like to provide further validation of the semantic capacity of generated contexts, and validate the underlying scoring function of \method (equation \ref{eqn:reflective_scoring}).

Specifically, \method is based on the notion that generated contexts can capture the main semantic aspects of a source text. To explicitly test this, we measure how well the reflective scoring function of equation \ref{eqn:reflective_scoring} captures semantic equivalence on the WMT18 metrics task \citep{ma2018results}. We specifically test on the segment-level evaluation, where the task is to rate the semantic equivalence of a number of machine generated translations to a reference human translation. Metrics/scoring functions are evaluated by their rank correlation (using a metric related to Kendall's Tau \cite{kendall1938new}) with human assessment of semantic equivalence. More details are available in the original task description.

In table \ref{tab:wmt18}, we present results on 3 language pairs: Chinese, German, and Estonian to English. Generally, higher correlation indicates a closer match with human judgement on which translations are closest in meaning to a reference translation. Metrics not significantly outperformed are bolded. We only include to-English translations as the language models used for \method are English. 

To apply equation \ref{eqn:reflective_scoring}, we generate contexts for the reference, and test how well each generated translation fits the reference-contexts. Specifically, we follow equation \ref{eqn:reflective_scoring}, taking the reference sentence as $s_{src}$ and measure the contextual similarity with each translation (taking translation to be $\hat{s}$ in each case). 

The high performance of our Reflective Scoring function (one of only 2 scoring functions bolded for all 3 pairs) indicates high agreement with human judges semantic equivalence between translations and reference. We are not aiming for state-of-the-art here, but rather to validate that generated contexts can represent full sentences well. This claim seems to be supported. 

\input{figs/wmt18}

\subsection{Ablations}

We include ablation studies for both the number of contexts generated $n_c$ (table \ref{tab:quora_ablation_n_C}) and whether weights $w$ are learned or set to be uniform (table \ref{tab:quora_ablation_weights}). In both cases, besides ablated aspects the experiment is conducted as in \S\ref{sec_experiments}.

For our ablation of generated contexts $n_c$ we investigate all 3 levels of novelty across 4 values of $n_c$: 6, 20, 40, 80, in table \ref{tab:quora_ablation_n_C}. We observe a broad trend of improving metrics with larger values of $n_c$, with the setting used in practice ($n_c = 80$) being a clear winner. An interesting aspect of this is that lower $n_c$ seems to force higher novelty. For $n_c = 20$, the lowest novelty achieved was 37.4, while this was 56.3 for $n_c = 6$. One potential cause for this is that the method cannot sufficiently capture the content of the source sentence with low $n_c$. With $n_c=80$, \method can effectively rewrite the input if it's allowed to, but this doesn't seem to be true for lower $n_c$.

In ablating weight learning, we consider 2 possible values of $n_c$: 6 and 10. This is because, without weight learning we must set $k_c = n_c$ as we cannot do weight pruning if weights are uniform. For $k_c$ much higher than this, the ensemble of equation \ref{eqn:rd} becomes prohibitively expensive to calculate. For both values of $n_c$ we found RD with weight learning outperforms uniform weights on the SARI metric. Interestingly, we found uniform weights resulted in a \textit{higher} novelty at $n_c = 6$ but a \textit{lower} novelty at $n_c = 10$, with a gap of almost 50. With weight learning, this gap is only about 8, indicating less variability in behavior when weight learning is used. 

\input{figs/quora_ablaction_n_c}
\input{figs/quora_ablation_weight_learning}


\section{Further Generations}
\label{app:examples}
See tables \ref{tab:anlg_gn_0} - \ref{tab:paraphrase_gen_1} for outputs of \method and a range of baselines on multiple example. We also include many generations of \method on the Quora paraphrasing dataset in table \ref{tab:RD_many_Gen}

\input{figs/RD_many_generations}
\input{figs/appendix_gen_anlg_0}
\input{figs/appendix_gen_anlg_1}
\input{figs/appendix_gen_anlg_2}


\input{figs/appendix_gen_paraphrase_0}
\input{figs/appendix_gen_paraphrase_1}



\input{figs/anlg_template}
\input{figs/paraphrasing_template}
